# Supplementary material for: Probabilistic Interval Analysis of Unreliable Programs
Source: arXiv:2404.16997 source file (2024-04-25)
Supplement: Supplementary file 1 [file abstract_partial_order_proof.tex]

We prove that $\sqsubseteq_M$ is a partial order relation as follows.

\begin{description}
\item[Reflexivity :] \hfill \\
	It's trivial to show that $\langle[a,b],p_{ab}\rangle\sqsubseteq_M\langle[a,b],p_{ab}\rangle$. It follows directly from the def.~\ref{abstract_order}.
\item[Transitivity :] \hfill \\
	$\langle[a,b],p_{ab}\rangle\sqsubseteq_M\langle[c,d],p_{cd}\rangle\qquad\qquad\mathrm{and}\qquad\qquad\langle[c,d],p_{cd}\rangle\sqsubseteq_M\langle[e,f],p_{ef}\rangle\hfill$ (Given)	
\begin{alignat}{2}
    [a,b]\sqsubseteq_{int}[c,d] &\qquad\land\qquad[c,d]\sqsubseteq_{int}[e,f]\label{eq:po1}\\
	p.m.f\Big(\langle[a,b],p_{ab}\rangle\Big)\geq\ p.m.f\Big(\langle[c,d],p_{cd}\rangle\Big) &\qquad\land\qquad p.m.f\Big(\langle[c,d],p_{cd}\rangle\Big)\geq\ p.m.f\Big(\langle[e,f],p_{ef}\rangle\Big)\label{eq:po2}
\end{alignat}
	
\noindent From eq.~\ref{eq:po1} we get $[a,b]\sqsubseteq_{int}[e,f]$ and from eq.~\ref{eq:po2} we get $p.m.f\Big(\langle[a,b],p_{ab}\rangle\Big)\geq\ p.m.f\Big(\langle[e,f],p_{ef}\rangle\Big)$.
	
	$\therefore\langle[a,b],p_{ab}\rangle\sqsubseteq_M\langle[e,f],p_{ef}\rangle$
\item[Anti-Symmetricity :] \hfill \\
	$\langle[a,b],p_{ab}\rangle\sqsubseteq_M\langle[c,d],p_{cd}\rangle\qquad\qquad\mathrm{and}\qquad\qquad\langle[c,d],p_{cd}\rangle\sqsubseteq_M\langle[a,b],p_{ab}\rangle\hfill$ (Given)
\begin{alignat}{2}
    [a,b]\sqsubseteq_{int}[c,d]\implies (c\leq a)\land (b\leq d)&\qquad\qquad\Big[\mathrm{from\ def.}~\ref{interval_def}\Big]\label{eq:po3}\\
	[c,d]\sqsubseteq_{int}[a,b]\implies (a\leq c)\land (d\leq b)&\qquad\qquad\Big[\mathrm{from\ def.}~\ref{interval_def}\Big]\label{eq:po4}\\
	p.m.f\Big(\langle[a,b],p_{ab}\rangle\Big)\geq p.m.f\Big(\langle[c,d],p_{cd}\rangle\Big)&\label{eq:po5}\\
	p.m.f\Big(\langle[c,d],p_{cd}\rangle\Big)\geq p.m.f\Big(\langle[a,b],p_{ab}\rangle\Big)&\label{eq:po6}
\end{alignat}

\noindent Combining eq.~\ref{eq:po3} and eq.~\ref{eq:po4} we get,\\
	$(c\leq a)\land (a\leq c)\implies a=c$ and\\
	$(b\leq d)\land (d\leq b)\implies b=d$\\
	$\therefore a=c,\ b=d$
	
\noindent From eq.~\ref{eq:po5} and eq.~\ref{eq:po6} we get,\\
	$p.m.f\Big(\langle[a,b],p_{ab}\rangle\Big)=p.m.f\Big(\langle[c,d],p_{cd}\rangle\Big)$\\
	$\Rightarrow \displaystyle\frac{p_{ab}}{b-a+1}=\frac{p_{cd}}{d-c+1}\hfill\Big[\mathrm{from\ def.}~\ref{pmf}\Big]$\\
	$\Rightarrow p_{ab}=p_{cd}\hfill\Big[\because a=c,\ b=d\quad\mathrm{and}\quad b-a+1\neq0\Big]$
	
	$\therefore\langle[a,b],p_{ab}\rangle=\langle[c,d],p_{cd}\rangle$
\end{description}
