# Supplementary material for: Probabilistic Interval Analysis of Unreliable Programs
Source: arXiv:2404.16997 source file (2024-04-25)
Supplement: Supplementary file 2 [file concrete_lub_glb_soundness_proof.tex]

Let, $\langle S_1,p_1\rangle$ and $\langle S_2,p_2\rangle$ are two elements in $L$. From eq.~\ref{eq:lub_L} we get the least upper bound $\langle S_u,p_u\rangle$ of $\langle S_1,p_1\rangle$ and $\langle S_2,p_2\rangle$ as
\begin{align}
\langle S_u,p_u\rangle=\langle S_1,p_1\rangle\bigsqcup_L\langle S_2,p_2\rangle=&\left\langle S_1\bigcup S_2,\textbf{min}(p_1,p_2)\right\rangle\nonumber&
\end{align}

\noindent Now, let $\langle S_c,p_c\rangle$ be any upper bound of both $\langle S_1,p_1\rangle$ and $\langle S_2,p_2\rangle$.

\noindent $\therefore \langle S_1,p_1\rangle\sqsubseteq_L\langle S_c,p_c\rangle\qquad and\qquad \langle S_2,p_2\rangle\sqsubseteq_L \langle S_c,p_c\rangle$

\noindent From def.~\ref{concrete_order} we get :
\begin{align*}
&S_1\subseteq S_c\ \bigwedge\ S_2\subseteq S_c\qquad\implies\qquad S_1\bigcup S_2\subseteq S_c&\\
&p_1\geq p_c\ \bigwedge\ p_2\geq p_c\qquad\implies\qquad \textbf{min}(p_1,p_2)\geq p_c&\\
\therefore\quad&\left\langle S_1\bigcup S_2, \textbf{min}(p_1,p_2)\right\rangle\qquad\sqsubseteq_L\qquad \langle S_c,p_c\rangle&\\
\Rightarrow\quad&\langle S_u,p_u\rangle\qquad\sqsubseteq_L\qquad \langle S_c,p_c\rangle&
\end{align*}

\noindent We have shown that $\langle S_u,p_u\rangle\sqsubseteq_L \langle S_c,p_c\rangle$, for any upper bound $\langle S_c,p_c\rangle$.

\noindent $\therefore \langle S_u,p_u\rangle$ is the least upper bound.

\noindent In a similar way we can give a proof of soundness for the greatest lower bound $\displaystyle\bigsqcap^L$ too.
