# Supplementary material for: Probabilistic Interval Analysis of Unreliable Programs
Source: arXiv:2404.16997 source file (2024-04-25)
Supplement: Supplementary file 6 [file concrete_partial_order_proof.tex]

We prove that $\sqsubseteq_L$ is a partial order relation as follows.

\begin{description}
\item[Reflexivity :] \hfill \\
	Reflexivity follows trivially from def.~\ref{concrete_order}. $\qquad\therefore\forall \langle S,p\rangle\in L\qquad\langle S,p\rangle\sqsubseteq_L\langle S,p\rangle$.
\item[Transitivity :] \hfill
\begin{alignat}{2}
    \langle S_1,p_1\rangle\sqsubseteq_L\langle S_2,p_2\rangle &\ \bigwedge\ \langle S_2,p_2\rangle\sqsubseteq_L\langle S_3,p_3\rangle\qquad\text{(given)}\nonumber\\
    S_1\subseteq S_2 &\ \bigwedge\ S_2\subseteq S_3\qquad\implies\qquad S_1\subseteq S_3\nonumber\\
    p_1\geq p_2 &\ \bigwedge\ p_2\geq p_3\qquad\implies\qquad p_1\geq p_3\nonumber
\end{alignat}
	
$\therefore \langle S_1,p_1\rangle\sqsubseteq_L\langle S_3,p_3\rangle$
\item[Anti-Symmetricity :] \hfill
\begin{alignat}{2}
    \langle S_1,p_1\rangle\sqsubseteq_L\langle S_2,p_2\rangle &\ \bigwedge\ \langle S_2,p_2\rangle\sqsubseteq_L\langle S_1,p_1\rangle\qquad\text{(given)}\nonumber\\
    S_1\subseteq S_2 &\ \bigwedge\ S_2\subseteq S_1\qquad\implies\qquad S_1=S_2\nonumber\\
    p_1\geq p_2 &\ \bigwedge\ p_2\geq p_1\qquad\implies\qquad p_1=p_2\nonumber
\end{alignat}

$\therefore \langle S_1,p_1\rangle=\langle S_2,p_2\rangle$
\end{description}
