# Supplementary material for: Probabilistic Interval Analysis of Unreliable Programs
Source: arXiv:2404.16997 source file (2024-04-25)
Supplement: Supplementary file 7 [file galois_connection_monotonicity_proof.tex]

From def.~\ref{gamma}, we have,

\begin{tabular}{@{\hspace{2mm}}rcl}
  $\GAMMA$$\Big(\big\langle[\ ],\ 1\big\rangle\Big)$ & = & $\Big\langle\big\{\ \big\},\ 1\Big\rangle=\perp_L$\\
  $\GAMMA$$\Big(\big\langle[a,\ b],\ p_{ab}\big\rangle\Big)$ & = & $\bigg\langle\bigg\{i\in\mathbb{Z}\ :\ a\leq i\leq b\bigg\},\ p.m.f\Big(\langle[a,b],p_{ab}\rangle\Big)\bigg\rangle$
\end{tabular}

\noindent Let, $\langle[a,b],p_{ab}\rangle$ and $\langle[c,d],p_{cd}\rangle$ be two elements in $M$, with $\langle[a,b],p_{ab}\rangle\sqsubseteq_M\langle[c,d],p_{cd}\rangle$\footnote{If $\quad\perp_M\sqsubseteq_M\langle[a,b],p_{ab}\rangle$, we trivially have $\quad$$\GAMMA$$\Big(\perp_M\Big)\sqsubseteq_L\ $$\GAMMA$$\Big(\langle[a,b],p_{ab}\rangle\Big)\quad$[$\ \because$$\GAMMA$$\Big(\perp_M\Big)=\perp_L$ is the least element in $\mathcal{L}$]}. We show that $\GAMMA$$\Big(\langle[a,b],p_{ab}\rangle\Big)\sqsubseteq_L\ $$\GAMMA$$\Big(\langle[c,d],p_{cd}\rangle\Big)$

\noindent$\because\langle[a,b],p_{ab}\rangle\sqsubseteq_M\langle[c,d],p_{cd}\rangle$, from def.~\ref{abstract_order} we have
\begin{flalign}
  &[a,b]\sqsubseteq_{int}[c,d]\qquad\qquad\text{and}\nonumber&&\\
  &p.m.f\big(\langle[a,b],p_{ab}\rangle\big)\geq p.m.f\big(\langle[c,d],p_{cd}\rangle\big)\label{eq:monotone1}&&
\end{flalign}
\begin{flalign}
  &\quad[a,b]\sqsubseteq_{int}[c,d]&\nonumber\\
  \Rightarrow &\quad c\leq a\bigwedge b\leq d&[\text{from def.}~\ref{interval_def}]\nonumber\\
  \Rightarrow &\quad\{i\in\mathbb{Z}\ |\ a\leq i\leq b\}\subseteq\{i\in\mathbb{Z}\ |\ c\leq i\leq d\}\label{eq:monotone2}&
\end{flalign}

\noindent From eq.~\ref{eq:monotone1} and eq.~\ref{eq:monotone2} we get, $\qquad$$\GAMMA$$\Big(\langle[a,b],p_{ab}\rangle\Big)\sqsubseteq_L\ $$\GAMMA$$\Big(\langle[c,d],p_{cd}\rangle\Big)$\hfill[using def.~\ref{concrete_order}]

\noindent This completes the proof that $\GAMMA$ is monotonic.

\noindent\rule{14cm}{0.1pt}

\noindent From def.~\ref{alpha}, we have,
\begin{align*}
\ALPHA\big(\langle S,p\rangle\big)= 
  \begin{cases} 
    \big\langle[\ ],\ 1\big\rangle=\perp_M        &        \langle S,p\rangle=\langle\phi,1\rangle=\perp_L\\
    \bigg\langle\Big[\mathcal{V}_m\Big(\langle S,p\rangle\Big),\ \mathcal{V}_M\Big(\langle S,p\rangle\Big)\Big],\ \mathbf{min}\bigg(1,\ p\cdot\Big(\mathcal{V}_M\Big(\langle S,p\rangle\Big)-\mathcal{V}_m\Big(\langle S,p\rangle\Big)+1\Big)\bigg)\bigg\rangle        &        \text{otherwise}
  \end{cases} 
\end{align*}

\noindent Now, suppose $\langle S_1,p_1\rangle$ and $\langle S_2,p_2\rangle$ are two elements in $L$, with $\langle S_1,p_1\rangle\sqsubseteq_L\langle S_2,p_2\rangle$ and $S_1\neq\phi$\footnote{If $\quad S_1=\phi$, we have $\langle S_1,p_1\rangle=\perp_L\sqsubseteq_L\langle S_2,p_2\rangle\ \Rightarrow\ $$\ALPHA$$\Big(\perp_L\Big)\sqsubseteq_M\ $$\ALPHA$$\Big(\langle S_2,p_2\rangle\Big),\quad[\ \because\ $$\ALPHA$$\Big(\perp_L\Big)=\langle[],1\rangle=\perp_M,\ $ the least element of $\mathcal{M}]$.}. We show that $\ALPHA$$\Big(\langle S_1,p_1\rangle\Big)\sqsubseteq_M\ $$\ALPHA$$\Big(\langle S_2,p_2\rangle\Big)$

\noindent $\because\langle S_1,p_1\rangle\sqsubseteq_L\langle S_2,p_2\rangle$, from def.~\ref{concrete_order}, we have,
\begin{flalign}
  &S_1\subseteq S_2\label{eq:monotone3}&&\\
  &p_1\geq p_2\label{eq:monotone4}&&
\end{flalign}

\noindent$\ALPHA$$\big(\langle S_1,p_1\rangle\big) = \bigg\langle\Big[\mathcal{V}_m\Big(\langle S_1,p_1\rangle\Big),\ \mathcal{V}_M\Big(\langle S_1,p_1\rangle\Big)\Big],\ \mathbf{min}\bigg(1,\ p_1\cdot\Big(\mathcal{V}_M\Big(\langle S_1,p_1\rangle\Big)-\mathcal{V}_m\Big(\langle S_1,p_1\rangle\Big)+1\Big)\bigg)\bigg\rangle\qquad$ and

\noindent$\ALPHA$$\big(\langle S_2,p_2\rangle\big) = \bigg\langle\Big[\mathcal{V}_m\Big(\langle S_2,p_2\rangle\Big),\ \mathcal{V}_M\Big(\langle S_2,p_2\rangle\Big)\Big],\ \mathbf{min}\bigg(1,\ p_2\cdot\Big(\mathcal{V}_M\Big(\langle S_2,p_2\rangle\Big)-\mathcal{V}_m\Big(\langle S_2,p_2\rangle\Big)+1\Big)\bigg)\bigg\rangle$\\

\noindent From eq.~\ref{eq:monotone3}, we get,
\begin{flalign}
&\quad\mathcal{V}_m\Big(\langle S_2,p_2\rangle\Big)\leq\mathcal{V}_m\Big(\langle S_1,p_1\rangle\Big)\ \bigwedge\ \mathcal{V}_M\Big(\langle S_1,p_1\rangle\Big)\leq\mathcal{V}_M\Big(\langle S_2,p_2\rangle\Big)&&\nonumber\\
\Rightarrow&\quad\Big[\mathcal{V}_m\Big(\langle S_1,p_1\rangle\Big),\ \mathcal{V}_M\Big(\langle S_1,p_1\rangle\Big)\Big]\ \sqsubseteq_{int}\ \Big[\mathcal{V}_m\Big(\langle S_2,p_2\rangle\Big),\ \mathcal{V}_M\Big(\langle S_2,p_2\rangle\Big)\Big]\qquad\qquad\text{[using def.~\ref{interval_def}]}&&\label{eq:monotone5}
\end{flalign}

\noindent From eq.~\ref{eq:monotone5}, we get,
  \begin{flalign}
    &\quad\mathcal{V}_M\Big(\langle S_1,p_1\rangle\Big)-\mathcal{V}_m\Big(\langle S_1,p_1\rangle\Big)+1\leq\mathcal{V}_M\Big(\langle S_2,p_2\rangle\Big)-\mathcal{V}_m\Big(\langle S_2,p_2\rangle\Big)+1&&\nonumber\\
    \Rightarrow&\quad\displaystyle\frac{1}{\mathcal{V}_M\Big(\langle S_1,p_1\rangle\Big)-\mathcal{V}_m\Big(\langle S_1,p_1\rangle\Big)+1}\geq\displaystyle\frac{1}{\mathcal{V}_M\Big(\langle S_2,p_2\rangle\Big)-\mathcal{V}_m\Big(\langle S_2,p_2\rangle\Big)+1}&&\label{eq:monotone6}
  \end{flalign}
  
\noindent$p.m.f\Big($$\ALPHA$$\big(\langle S_i,p_i\rangle\big)\Big) = \mathbf{min}\left(p_i,\displaystyle\frac{1}{\mathcal{V}_M\Big(\langle S_i,p_i\rangle\Big)-\mathcal{V}_m\Big(\langle S_i,p_i\rangle\Big)+1}\right)\qquad\forall i\in\{1,2\}$

\noindent Now, depending upon the values of $\quad p.m.f\Big($$\ALPHA$$\big(\langle S_1,p_1\rangle\big)\Big)\quad$ and $\quad p.m.f\Big($$\ALPHA$$\big(\langle S_2,p_2\rangle\big)\Big),\quad$ we have 4 different cases to consider.

\begin{description}
  \item[Case 1 :] $p.m.f\Big($$\ALPHA$$\big(\langle S_1,p_1\rangle\big)\Big)=p_1\qquad$ and $\qquad p.m.f\Big($$\ALPHA$$\big(\langle S_2,p_2\rangle\big)\Big)=p_2$ \hfill \\
    From eq.~\ref{eq:monotone4}, it's obvious that $\qquad p.m.f\Big($$\ALPHA$$\big(\langle S_1,p_1\rangle\big)\Big)\geq p.m.f\Big($$\ALPHA$$\big(\langle S_2,p_2\rangle\big)\Big)$
  
  \item[Case 2 :] $p.m.f\Big($$\ALPHA$$\big(\langle S_1,p_1\rangle\big)\Big)=p_1\qquad$ and $\qquad p.m.f\Big($$\ALPHA$$\big(\langle S_2,p_2\rangle\big)\Big)=\displaystyle\frac{1}{\mathcal{V}_M\Big(\langle S_2,p_2\rangle\Big)-\mathcal{V}_m\Big(\langle S_2,p_2\rangle\Big)+1}$ \hfill \\
    
    $\because\ p.m.f\Big($$\ALPHA$$\big(\langle S_2,p_2\rangle\big)\Big)=\displaystyle\frac{1}{\mathcal{V}_M\Big(\langle S_2,p_2\rangle\Big)-\mathcal{V}_m\Big(\langle S_2,p_2\rangle\Big)+1}$
    \begin{flalign*}
      \Rightarrow&\quad p_2\geq\frac{1}{\mathcal{V}_M\Big(\langle S_2,p_2\rangle\Big)-\mathcal{V}_m\Big(\langle S_2,p_2\rangle\Big)+1}&&\\
      \Rightarrow&\quad p_1\geq\frac{1}{\mathcal{V}_M\Big(\langle S_2,p_2\rangle\Big)-\mathcal{V}_m\Big(\langle S_2,p_2\rangle\Big)+1} & \text{[from eq.~\ref{eq:monotone4}]} &
    \end{flalign*}
  $\therefore\ p.m.f\Big($$\ALPHA$$\big(\langle S_1,p_1\rangle\big)\Big)\geq p.m.f\Big($$\ALPHA$$\big(\langle S_2,p_2\rangle\big)\Big)$
  
  \item[Case 3 :] $p.m.f\Big($$\ALPHA$$\big(\langle S_1,p_1\rangle\big)\Big)=\displaystyle\frac{1}{\mathcal{V}_M\Big(\langle S_1,p_1\rangle\Big)-\mathcal{V}_m\Big(\langle S_1,p_1\rangle\Big)+1}\qquad$ and $\qquad p.m.f\Big($$\ALPHA$$\big(\langle S_2,p_2\rangle\big)\Big)=p_2$ \hfill \\
  
  $\because\ p.m.f\Big($$\ALPHA$$\big(\langle S_2,p_2\rangle\big)\Big)=p_2$
    \begin{flalign*}
      \Rightarrow&\quad\frac{1}{\mathcal{V}_M\Big(\langle S_2,p_2\rangle\Big)-\mathcal{V}_m\Big(\langle S_2,p_2\rangle\Big)+1}\geq p_2&&\\
      \Rightarrow&\quad\frac{1}{\mathcal{V}_M\Big(\langle S_1,p_1\rangle\Big)-\mathcal{V}_m\Big(\langle S_1,p_1\rangle\Big)+1}\geq p_2 & \text{[from eq.~\ref{eq:monotone6}]} &
    \end{flalign*}
  $\therefore\ p.m.f\Big($$\ALPHA$$\big(\langle S_1,p_1\rangle\big)\Big)\geq p.m.f\Big($$\ALPHA$$\big(\langle S_2,p_2\rangle\big)\Big)$
  
  \item[Case 4 :] $p.m.f\Big($$\ALPHA$$\big(\langle S_i,p_i\rangle\big)\Big)=\displaystyle\frac{1}{\mathcal{V}_M\Big(\langle S_i,p_i\rangle\Big)-\mathcal{V}_m\Big(\langle S_i,p_i\rangle\Big)+1}\qquad\forall i\in\{1,2\}$ \hfill \\
    From eq.~\ref{eq:monotone6}, it's obvious that $\qquad p.m.f\Big($$\ALPHA$$\big(\langle S_1,p_1\rangle\big)\Big)\geq p.m.f\Big($$\ALPHA$$\big(\langle S_2,p_2\rangle\big)\Big)$
\end{description}

\noindent So, in all the 4 cases, $\quad p.m.f\Big($$\ALPHA$$\big(\langle S_1,p_1\rangle\big)\Big)\geq p.m.f\Big($$\ALPHA$$\big(\langle S_2,p_2\rangle\big)\Big)$. This result along with eq.~\ref{eq:monotone5} proves that $\ALPHA$$\Big(\langle S_1,p_1\rangle\Big)\sqsubseteq_M\ $$\ALPHA$$\Big(\langle S_2,p_2\rangle\Big)$.

\noindent This completes the proof that $\ALPHA$ is monotonic.
